# Supplementary material for: Density of states in neural networks: an in-depth exploration of learning in parameter space
Source: arXiv:2409.18683 ancillary file (2024-09-27)
Supplement: Supplementary file 1 [file supp.pdf]

# Supplementary material to
# *Density of states in neural networks: an in-depth exploration of learning in parameter space*

Margherita Mele,[1,2] Roberto Menichetti,[1,2] Alessandro Ingrosso,[3,*] and Raffaello Potestio[1,2,†]

[1] *Physics Department, University of Trento, via Sommarive, 14 I-38123 Trento, Italy*
[2] *INFN-TIFPA, Trento Institute for Fundamental Physics and Applications, I-38123 Trento, Italy*
[3] *Donders Institute for Brain, Cognition and Behaviour, Radboud University, Nijmegen, The Netherlands*

(Dated: September 26, 2024)

## I. ADDITIONAL DETAILS ON THE DATASETS

The *synthetic* datasets represent isotropic distributions in $N$ dimensions, with two classes whose mean vectors are derived from orthogonal normalized vectors sampled from a univariate normal distribution. Specifically, consider two such vectors in $N$ dimensions, with components sampled from a univariate normal distribution:

$$m_c = \left\{ \frac{m_i^c}{\|m_c\|} \right\}_{i=1}^{N} \quad \text{with} \quad m_i^c = \mathcal{N}(0,1) \text{ and } c \in \{1,2\} \tag{1}$$

The mean vectors of the two classes are defined as follows:

$$\begin{cases} \mu_1 \equiv \Delta\mu \cdot m_1 & \text{class 1} \\ \mu_2 \equiv \Delta\mu \cdot [\lambda \cdot m_1 + (1-|\lambda|) \cdot m_2] & \text{class 2} \end{cases} \tag{2}$$

Here, $\lambda \in [-1,1]$ and $\Delta\mu \in [0,+\infty)$ are the morphing parameters controlling the angle between the two mean vectors and the inter-class separation, respectively. When $\lambda = 1$, the two vectors are parallel ($\mu_1 = \mu_2$) and the inter-class separation is zero ($||\mu_1 - \mu_2|| = 0$). For $\lambda = 0$, the two vectors are orthogonal since $m_1 \perp m_2$, and the inter inter-class distance is $||\mu_1 - \mu_2|| = \Delta\mu\sqrt{2}$. Finally, when $\lambda = -1$, the two mean vectors are antiparallel ($\mu_1 = -\mu_2$) and the inter-class separation is $||\mu_1 - \mu_2|| = 2\Delta\mu$. For a generic value of $\lambda$, the inter-class distance is given by:

$$||\mu_1 - \mu_2|| = \Delta\mu\sqrt{(1-\lambda)^2 + (1-|\lambda|)^2} \tag{3}$$

The angle between the mean vectors is defined by:

$$\theta = \arccos \frac{\mu_1 \cdot \mu_2}{||\mu_1|| ||\mu_2||} = \arccos \frac{\lambda}{\sqrt{\lambda^2 + (1-|\lambda|)^2}} \tag{4}$$

## II. ADDITIONAL DETAILS ON THE WANG-LANDAU ALGORITHM

This supplementary section provides an in-depth explanation of the implementation details and parameters used in the Wang-Landau (WL) sampling method as applied in our study.

At each stage of the WL simulation, the nature of the move—local or global—is determined by a random number $c \in (0,1)$. Specifically, if $c < 0.8$, the move is local, meaning that one of the $N$ components of the weight vector $W$ is randomly selected and flipped to generate $W'$. Conversely, when $c > 0.8$, another random number is drawn to determine the number $n \leq N$ of components to be changed. These $n$ components are then randomly selected and flipped.

The flatness condition is a crucial aspect of the WL algorithm, ensuring the uniformity of the histogram of visited energy levels. This condition is typically defined by the requirement that for each value of energy $E$, the histogram value $H_k(E)$ must not deviate significantly from the mean value $\langle H_k \rangle$. Mathematically, this is expressed as:

$$p_{flat} \times \langle H_k \rangle < H_k(E) < (2 - p_{flat}) \times \langle H_k \rangle,$$

where $p_{flat}$ is a predefined flatness parameter.

In the simulations performed in our study, we set $p_{flat}$ to 0.9. The flatness condition for the visited energy levels was checked every 800 Monte Carlo (MC) moves. The iterative simulation scheme was continued until the modification factor $F$ decreased below the predefined final value, $F_{end} = \ln(f_{end}) = 10^{-6}$.

By adhering to these detailed procedures and parameter settings, the WL scheme ensures a comprehensive exploration of the energy landscape, ultimately leading to an accurate determination of the density of states $\Omega(E)$ for the network under study.

* alessandro.ingrosso@donders.ru.nl
† raffaello.potestio@unitn.it

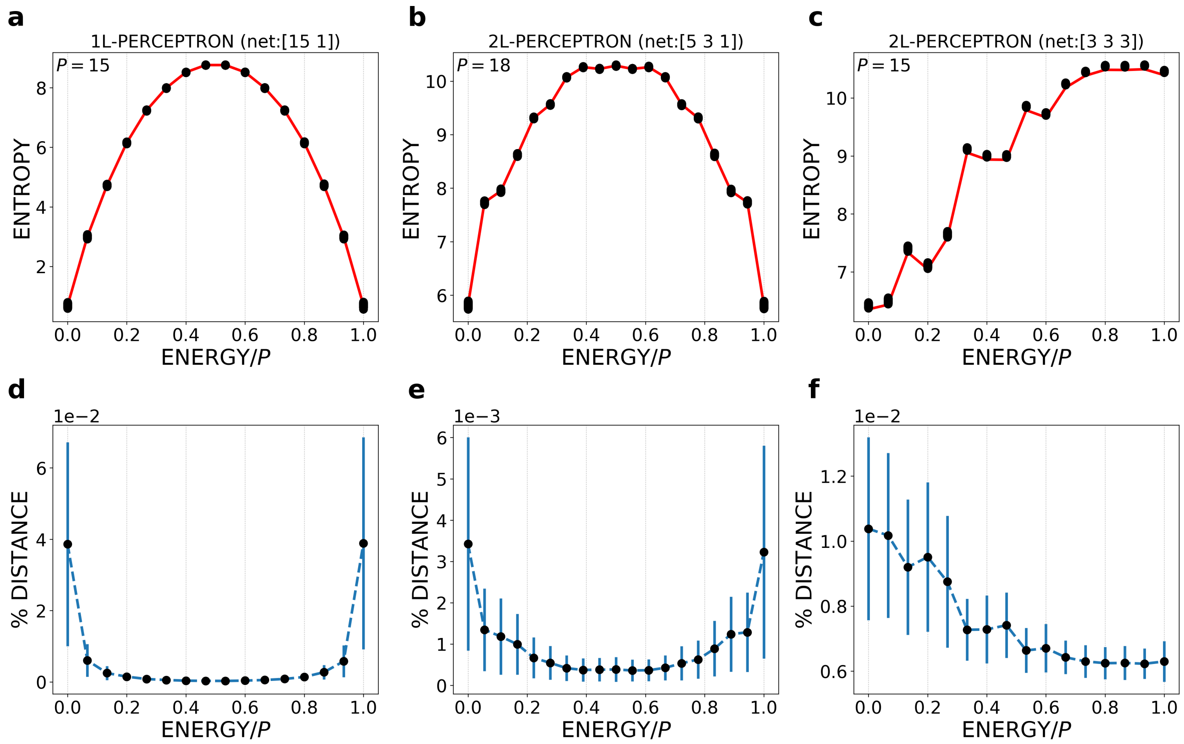


**Figure 1**. Comparison of the true entropy curve to the output of the Wang-Landau algorithm across different network architectures. For each architecture, 500 independent simulations are performed on the same dataset composed of P data points. The upper panels (a-c) compare the true entropy curve (red-solid line) with the sampled ones (black points). The lower panels (d-f) show the mean percentage difference between the true and sampled entropy curves, with associated errors. **(a)** Single-layer perceptron with 15 input neurons and $P = 15$. **(b)** one-hidden layer network for binary classification with 5 input neurons, 3 hidden neurons and $P = 18$. **(c)** One-hidden layer network for multi-class classification with 3 input neurons, 3 hidden neurons, 3 output neurons and $P = 15$. The corresponding lower panels (d, e, f) illustrate the mean value of the percentage difference between the true and sampled entropy curves with the associated error bars.

## III. VALIDATION AND SCALING ANALYSIS

In this section, we aim to validate the accuracy of the Wang-Landau (WL) sampling method in estimating the entropy curves for small neural network systems. Additionally, we perform a scaling analysis to assess how the algorithm's convergence time increases with respect to network size and learning complexity.

### A. Validation of entropy estimation

To verify the accuracy of the entropy curves obtained by Wang-Landau (WL) sampling, systems with small dimensions were used to ensure that the configuration space was small enough to exhaustively list all states and calculate their associated energies. This approach allowed an exact calculation of the microcanonical entropy curve $S_T(E)$, which could then be compared with the WL-estimated curve $S_{WL}(E)$. Three different neural network architectures were analysed: (i) a single-layer perceptron with 15 input neurons, (ii) a one-hidden layer network with 5 input neurons and 3 hidden neurons for binary classification (one output neuron), and (iii) a one-hidden layer network for multi-class classification with 3 input neurons, 3 hidden neurons and 3 output neurons. A data set of $P$ elements was generated using an identical teacher network for each architecture: $P = 15$ for the single-layer perceptron, $P = 18$ for the one-hidden layer network in binary classification, and $P = 15$ for the one-hidden layer network in multi-class classification. For each scenario, 500 independent WL simulations were performed and the results are shown in Figure 1. The top part of the figure shows the real entropy curves (continuous red line) alongside the 500 sampled curves (black points), highlighting a general agreement between the WL-derived and real curves. To quantify this agreement, the percentage distance between each sampled curve and the real curve was calculated using the formula:

$$\text{dist}\left(S_{WL}(E), S_T(E)\right) = \frac{|S_{WL}(E) - S_T(E)|}{S_T(E)} \tag{5}$$

The average value of this distance, together with the associated standard deviation, is shown in the bottom part of Figure 1. In all cases, the average percentage distance is consistently less than $7e-2$. These results confirm the reliability of WL sampling in accurately estimating entropy curves.

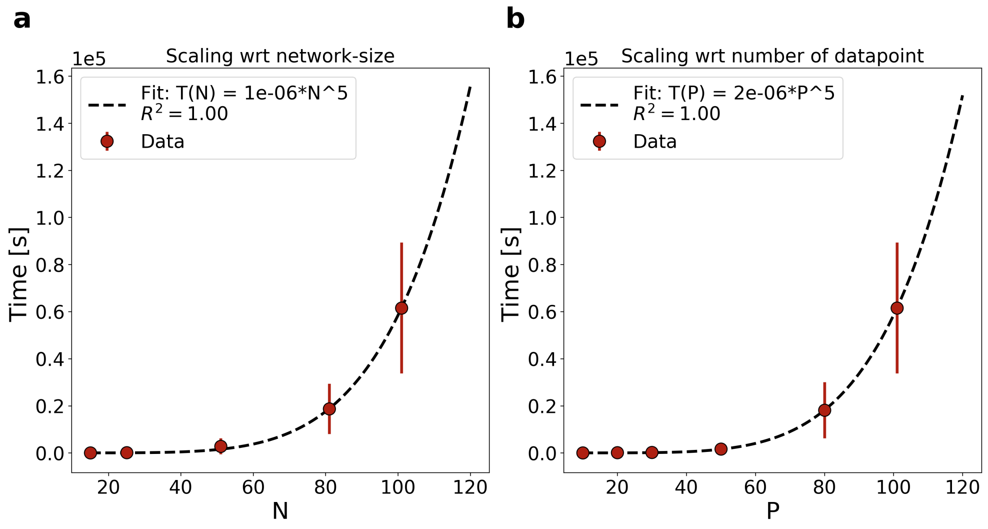


**Figure 2**. Convergence time of the Wang-Landau algorithm executed on a single core as a function of network size and learning complexity. **(a)** The scaling of convergence time with respect to the number of neurons $N$ in a single-layer perceptron, at a fixed learning complexity $\alpha = \frac{P}{N} = 1$. For each value of $N$, 7 independent datasets were generated, and for each dataset, 50 independent simulations were performed. The data points represent the mean convergence time, and the dashed line represents the fitted curve with $T(N) = 10^{-6}N^5$. **(b)** The convergence time as a function of the learning complexity $\alpha$, at a fixed number of neurons $N = 100$. Similarly, 7 datasets were generated for each value of $P$, and 50 independent simulations were conducted per dataset. The fitted curve is $T(P) = 2 \times 10^{-6}P^5$.

### B. Scaling analysis of the Wang-Landau algorithm

The performance of the Wang-Landau (WL) algorithm was further analyzed by examining its convergence time as a function of two key parameters: the number of neurons in a single-layer perceptron and the learning complexity. This scaling analysis was performed to assess how the algorithm's computational cost grows with increasing network size and data complexity.

The first analysis focused on the dependence of convergence time on the number of neurons $N$ in a single-layer perceptron, while keeping the learning complexity $\alpha = \frac{P}{N} = 1$ constant. For each value of $N$, 7 independent datasets were generated, and 50 independent WL simulations were conducted per dataset. The average convergence times were recorded and are plotted in Figure 2. The results indicate that the convergence time scales approximately as $T(N) \sim 10^{-6}N^5$, suggesting a power-law dependence on the number of neurons.

In the second analysis, the convergence time was studied as a function of the learning complexity $\alpha = \frac{P}{N}$ for a fixed number of input neurons $N = 100$. Again, 7 independent datasets were generated for each value of $P$, and 50 independent WL simulations were run per dataset. The results, shown in Figure 2, indicate that the convergence time scales as $T(P) \sim 2 \times 10^{-6}P^5$. This behavior reflects the growing computational cost as the problem complexity increases with more data points $P$.

Overall, these scaling analyses reveal that the Wang-Landau algorithm exhibits a computational cost that grows polynomially with both the number of neurons and the learning complexity, with exponents of approximately 5 in both cases. This insight is crucial for understanding the limitations of the WL algorithm when applied to large neural networks or complex datasets, providing valuable guidance for future implementations and optimizations.

## IV. GAUSSIAN FIT

In this subsection, we analyze the density of states (DoS) curves for binary classification using a single-layer perceptron. Our goal is to determine whether the distribution of states obtained from classifying independent and identically distributed (i.i.d.) data follows a Gaussian distribution. Figure 3 presents the DoS curves for different numbers of input neurons, $N$, along with a Gaussian fit, with the fit parameters—the standard deviation ($\sigma$) and the mean ($\mu$) of the Gaussian distribution— indicated in the upper left corner. Additionally, the goodness of fit is measured by the coefficient $R^2$, also shown in the upper left corner of each panel. The $R^2$ value indicates how well the Gaussian model represents the observed DoS, with values closer to 1 signifying a better fit. Although the density of states is not continuous in the cases studied, the DoS approaches a continuous distribution in the thermodynamic limit, where both $N$ and the number of patterns $P$ increase indefinitely while maintaining a fixed ratio. This analysis demonstrates that, under these conditions, the DoS curves closely align with a Gaussian distribution, supporting the use of Gaussian models to describe the statistical behavior of single-layer perceptrons in binary classification tasks with i.i.d. data.

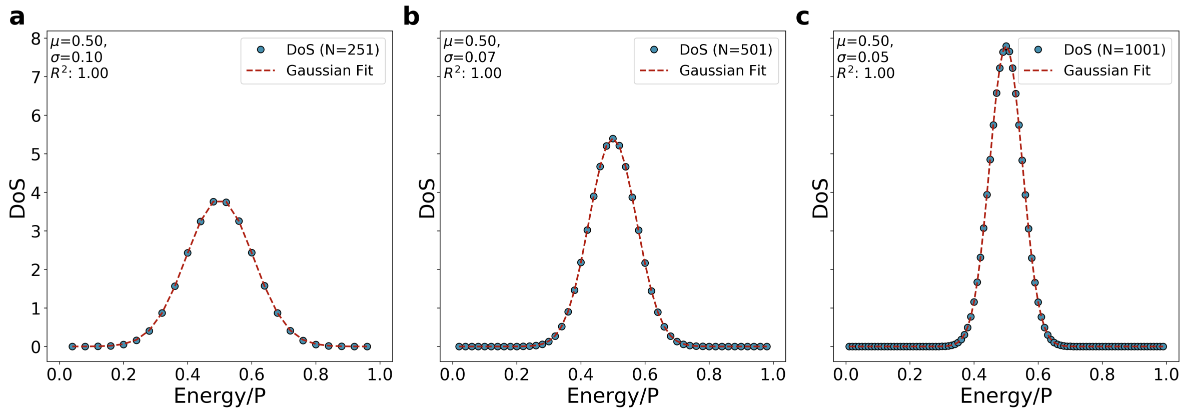


**Figure 3**. Density of States Curves for Binary Classification by a Single-Layer Perceptron and Gaussian Fit. Each panel presents the density of states for binary classification of random data using a single-layer perceptron with different numbers of input layer neurons, $N$ as specified in the legend. The top left corner of each plot provides the parameters of the Gaussian fit, including the standard deviation ($\sigma$) and the mean ($\mu$), as well as the coefficient of determination ($R^2$).

## V. FASHION-MNIST

This section provides an analysis of a subset of the FashionMNIST dataset, focusing on the binary classification of T-shirt/top and trouser images, to assess the generality of trends observed in the presence of different class imbalances. As shown in Figure 4, the results mirror those presented in the main text, reinforcing the critical role of class imbalance in modelling density of states (DoS) curves.

At lower complexity ($P/N = 0.1$), the DoS reveals a clear symmetry: as class imbalance increases, the peaks shift progressively from the center of the spectrum, regardless of which class is predominant. This pattern is maintained even at higher complexity ($P/N = 0.5$), where the separation of the peaks becomes more pronounced with imbalance. In both cases, the location of these peaks reflects the degree of imbalance, with the largest deviations from balance showing the most extreme shifts.

The correlation between peak energy and imbalance is further highlighted in the scatter plot, where the absolute difference $|0.5 - P_1/P|$ captures the relationship between class distribution and peak shift. This trend holds across different learning complexities, demonstrating the robustness of this behavior. These results on FashionMNIST corroborate our findings in the main text and emphasize that the DoS landscape is significantly influenced by structured data, with class imbalance driving non-trivial modifications in the energy spectrum.

## VI. GAUSSIAN CLONES

In order to better understand the role of statistical properties of data in learning dynamics, we introduced Gaussian clones, which are synthetic datasets that approximate real-world data with progressively higher moments retained. These clones allow us to examine the influence of specific data properties, such as the mean and covariance, on the learning process. The main purpose of using Gaussian clones is to isolate and control key statistical properties, offering insights into how these properties shape the network's performance. In particular, we constructed two main types of clones: the GM clone (Gaussian Mixture), which captures both the mean and full covariance matrix of each class, and the 2isoGM clone (isotropic Gaussian Mixture), a simplified version where only the mean vectors of the classes are preserved, and the variance is set equal across the two classes. This enables us to decouple the effect of higher-order cumulants and focus exclusively on first- and second-order statistics.

In both approximation, for each class the data are sampled form a Gaussin $\mathcal{N}(\mu_c \Delta\mu, \Sigma)$, where $\mu_c$ is the class-specific mean vector in an $N$-dimensional space, $\Delta\mu$ is a positive scalar parameter and $\Sigma$ is the covariance matrix:

$$\Sigma_{ij} = \begin{cases} \langle x_i - \langle x_i \rangle \rangle \langle x_j - \langle x_j \rangle \rangle & \text{GM} \\ v\, \delta_{ij} & \text{2isoGM} \end{cases} \quad (6)$$

$\delta_{ij}$ is the Kronecker delta, and $v = \sqrt{v_1 v_2}$ is the geometric mean of the variance of the two classes. In the GM clone, the full covariance matrix preserves the real feature correlations of the data, while in the 2isoGM clone, these correlations are ignored, and the variance structure is simplified to be isotropic.

By analyzing the results across different inter-class separations, i.e., for different value of $\Delta\mu$, we observed that the DoS curves from the Gaussian clones exhibited properties closely aligned with those seen in real datasets. In particular, if one is interested in the location of the maximum of the DoS, the structure of the covariance matrix does not seem to play a crucial role. The primary factor influencing the peak location is instead the separation between class means and the angle between the two mean vectors, which in the case of real datasets always falls below 90° (Figure 5.a). Furthermore, the location of the peak is modified by

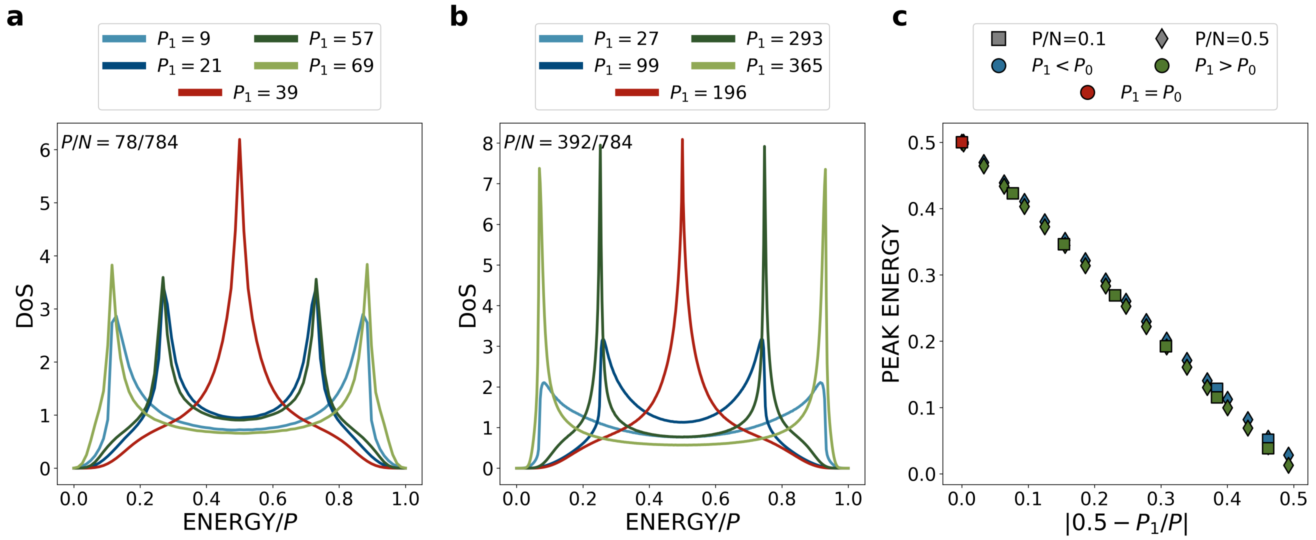


**Figure 4**. Density of states analysis for binary classification of FashionMNIST images (T-shirt/top and Trouser) under various class imbalances. (a) Density of states at a fixed learning complexity of $P/N = 0.1$, showing the distribution for different class imbalances. The legend indicates the number of elements in class 1 ($P_1$). Perfect class balance is achieved when $P_1 = P_0 = P/2$ (red curve). Larger deviations from this value indicate greater class imbalance. Blue curves represent a predominance of class 0, while green curves represent a predominance of class 1; the lighter the color, the greater the class imbalance. (b) Density of states at a higher learning complexity of $P/N = 0.5$, showing similar trends with varying class imbalances. (c) Peak energy values plotted against the absolute difference $|0.5 - P_1/P|$, highlighting the correlation between peak energy and class imbalance. Blue points indicate a predominance of class 0, while green points indicate a predominance of class 1. Red points represent perfect balance ($P_1 = P_0$). Results are shown for two values of learning complexity: $P/N = 0.1$ (squares) and $P/N = 0.5$ (diamonds).

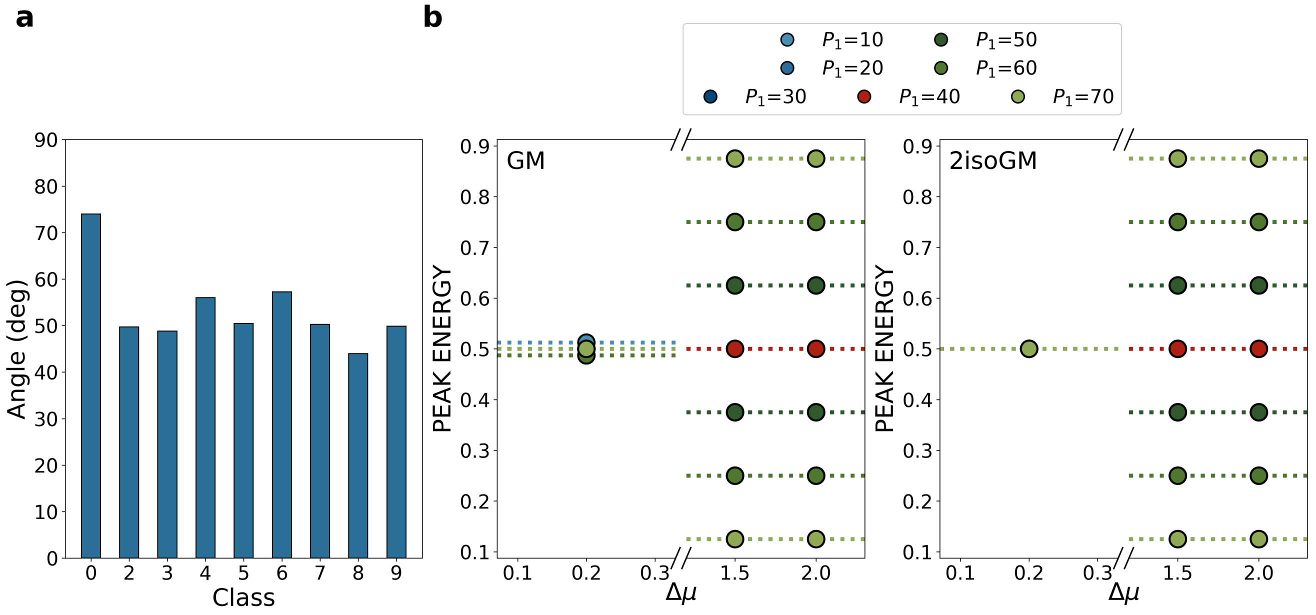


**Figure 5**. **(a)** Angle between the mean vector of class 1 and the mean vectors of other classes in the MNIST dataset, as indicated on the x-axis. **(b)** Peak location of the DoS plotted against the inter-class separation distance $\Delta\mu$ for different values of class imbalance, as shown in the legend. Results are obtained from 9 different binary classification problems, comparing MNIST class 1 against each of the other MNIST classes. Red points indicate balanced classes, while blue and green points represent unbalanced classes, with lighter colors corresponding to greater imbalance. The two panels differ in the approximation used for the covariance matrix: Gaussian Mixture (GM, left) and isotropic Gaussian Mixture (2isoGM, right) clones.

class unbalancing when the two classes are *far apart* ($\Delta\mu \gg 1$). In contrast, when the classes are *very close* ( $\Delta\mu \ll 1$), unbalancing has little effect on the peak location. This trend is identical in both GM and 2isoGM clones, suggesting that the structure of the covariance matrix does not play a predominant role in shaping this feature (Figure 5.b).
